# Supplementary material for: Characterizing EOSIO Blockchain
Source: arXiv:2002.05369 source file (2020-02-13)
Supplement: Supplementary file 1 [file appendix.tex]

\section{appendix}
